# Supplementary material for: Purifying electron spectra from noisy pulses with machine learning using synthetic Hamilton matrices
Source: arXiv:1908.02600 ancillary file (2020-03-12)
Supplement: Supplementary file 1 [file denoise-suppl.pdf]

# Supplement “Purifying electron spectra from noisy pulses with machine learning using synthetic Hamilton matrices”

Sajal K Giri, Ulf Saalmann, and Jan M Rost

Technical details for laser pulses, the propagation of the time-dependent Schrödinger equation and the training of artificial neural networks are provided. Parameters for the numerical calculations are specified.

## 1 Partial-coherence method

In order to create fluctuating pulses we apply the so-called partial-coherence method (PCM), which has been devised to simulate pulses from free-electron laser (FEL) sources [1]. Thereby a fluctuating (or noisy) pulse is given by

$$f_l(t) = N_l\, G(t)\, \mathcal{F}^{-1}\!\left[\mathrm{e}^{\mathrm{i}\phi_l(\omega)}\mathcal{F}[g(t)\cos(\omega_* t)]\right], \tag{S1a}$$

$$G(t) = \mathrm{e}^{-2\ln 2\, t^2/T^2} \quad \text{and} \quad g(t) = \mathrm{e}^{-t^2/\tau^2}, \tag{S1b}$$

with $\omega_*$ the carrier frequency. $\mathcal{F}$ and $\mathcal{F}^{-1}$ denotes the Fourier and the inverse Fourier transform, respectively. The actual noise realization, indicated by the index $l$, is given by random spectral phases $\phi_l$, uniformly distributed in the range of $-\pi \ldots +\pi$. For $\phi(\omega) = 0$ and $\tau \to 0$ we get an ideal Gaussian pulse — here the reference pulse $f_{\text{ref}}(t)$. The two Gaussians, defined in Eq. (S1b), appear in the pulse expression (S1a) inside and outside the Fourier transforms and serve different purposes. On one hand, $g(t)$ quantifies the time scale of the fluctuations[1] by means of the coherence time $\tau$. On the other side, $G(t)$ is a masking function in time that fixes the typical pulse duration $T$, which would be otherwise arbitrarily long. Thus $\tau \ll T$ implies strongly fluctuating pulses, which is the typical case at X-ray free-electron laser as, e. g., the European XFEL [2]. The pre-factor $N_l$ guarantees that the pulse energy of the fluctuating pulse is the same as the one of the reference pulse: $\int \mathrm{d}t\, f_l{}^2(t) = \int \mathrm{d}t\, f_{\text{ref}}{}^2(t)$. This “normalization” is the only difference to the standard PCM [1].

For the propagation of the time-dependent Schrödinger equation, cf. Sect. 3 below, we need the time dependent vector potential $A_l(t)$ at equidistant instants of time $t_\eta = \eta\, \delta t$ with $\eta = -\eta_{\max} \cdots + \eta_{\max}$. For obtaining $A_l(t_\eta)$ we have chosen maximum time $t_{\max} = -t_{\min} = 3{,}000$ a.u. and $\eta_{\max} = 2^{16}$ (thereby $\delta t \approx 0.046$ a.u.), did a fast Fourier transformation FFT, created $2\eta_{\max}$ random phases $\phi_\eta$ uniformly between $-\pi$ and $+\pi$, and did finally an inverse FFT.

## 2 Synthetic Hamilton matrices and creation of training/validation data

In order to create a sufficient amount of training data (we calculate $10^7$ time-dependent Schrödinger equations) we resort to Hamilton matrices based on an 1-dimensional model system. The starting point is the Hamilton operator

$$\widehat{H}(t) = -\frac{1}{2}\frac{\mathrm{d}^2}{\mathrm{d}x^2} - \frac{1}{\sqrt{x^2+1/2}} + A(t)\,\mathrm{i}\frac{\mathrm{d}}{\mathrm{d}x}, \tag{S2}$$

for which we define numerically on a grid ($x_j = j\Delta x$, with $\Delta x = 0.1$ a.u. and $x_{\max} = 500$ a.u.) all eigenstates $\widehat{H}\varphi_\alpha = \varphi_\alpha \widetilde{E}_\alpha$ with $\widetilde{E}_\alpha \le E_{\max} \approx 48$ eV, resulting in 600 eigenstates. By means of these states, we build the (600×600) Hamilton matrix

$$\widetilde{H}_{\alpha\beta}(t) = \widetilde{E}_\alpha\, \delta_{\alpha\beta} + A(t)\, \widetilde{V}_{\alpha\beta} \qquad \text{with} \quad \widetilde{V}_{\alpha\beta} \equiv \left\langle \varphi_\alpha \middle| \mathrm{i}\tfrac{\mathrm{d}}{\mathrm{d}x} \middle| \varphi_\beta \right\rangle. \tag{S3}$$

[1] One might consider other functions $g(t)$, e. g. [3], $g_{\mathrm{s}}(t) = \operatorname{sech}(\pi t/\sqrt{2}\tau)$ or $g_{\mathrm{e}}(t) = \exp(-2|t|/\tau)$. All three have the same coherence time, but different decay characteristics. We have tested all three noise types. Since they did not show any qualitative difference in terms of predictability of spectra, we present only results for the Gaussian-type noise (S1b).

This is a model of a 1-dimensional “helium atom”, since the ground-state energy $E_0 = -24.2\,\text{eV}$ is close to the ionization potential of real helium (24.6 eV).

As we want to train the network for “arbitrary” quantum systems, we create synthetic Hamilton matrices by randomly changing energies $\widetilde{E}_\alpha$ and matrix elements $\widetilde{V}_{\alpha\beta}$ in the following way

$$E_\alpha = 3^{[\xi_1-\gamma]}\widetilde{E}_\alpha \qquad \text{for } \widetilde{E}_\alpha<0,\ \alpha>0, \tag{S4a}$$

$$V_{0\alpha} = 3^{\xi_2}\widetilde{V}_{0\alpha} \qquad \text{for } \widetilde{E}_\alpha<0, \tag{S4b}$$

$$V_{\alpha\beta} = 3^{\xi_3}\widetilde{V}_{\alpha\beta} \qquad \text{for } \widetilde{E}_\alpha<0,\ \widetilde{E}_\beta>0, \tag{S4c}$$

$$V_{\alpha\beta} = 3^{\xi_4}\widetilde{V}_{\alpha\beta} \qquad \text{for } \widetilde{E}_\alpha>0,\ \widetilde{E}_\beta>0, \tag{S4d}$$

with four uniform random numbers $\xi_1 = [-1, +1.1]$, $\xi_2 = [-2, +2]$, and $\xi_{3,4} = [-1, +1]$. Thereby we modify the bound-state energies (S4a) and the couplings between ground and bound states (S4b), between bound and free states (S4c) and among free states (S4d), respectively. With $\gamma = 0.88$ and $\xi_1 = 0$ the energy difference between ground and excited state is equal to the central laser frequency $\omega_*$, i. e. $E_1 - E_0 = \omega_*$.

## 3 Propagation of the time-dependent Schrödinger equation (TDSE)

### “1D” systems for training data

Typically the propagation of the TDSE is done in fixed time steps $\delta t$ over which the Hamilton matrix is assumed to be constant, i. e. one step is taken by

$$\psi_\alpha(t+\delta t) = \sum_\beta U_{\alpha\beta}(t+\delta t, t)\psi_\beta(t), \tag{S5a}$$

$$U_{\alpha\beta}(t+\delta t, t) = \mathrm{e}^{-\mathrm{i}H_{\alpha\beta}(t+\delta t/2)\,\delta t}, \tag{S5b}$$

with $U_{\alpha\beta}$ the matrix representation of the (unitary) time-evolution operator.

In order to improve efficiency (considerably) we refrain from using a fixed time step, but rather discretize the laser pulse with a given step size in the *vector potential* $A(t)$. With $\delta A$ the step height, we can find intervals of time $t = t_j^{\text{beg}} \ldots t_j^{\text{end}}$ for which $\lfloor A(t)/\delta A \rceil = j$, with $\lfloor \ldots \rceil$ denoting the nearest integer. Now we have variable time steps, in which the assumption of constant values of the vector potential is a good approximation by construction. Such a discretization perfectly adapts to any pulse. Figure S1 shows this discretization of the pulse.

Since there could be more than one interval for a given $j$ we pre-diagonalize the matrices

$$H^j_{\alpha\beta} = E_\alpha \delta_{\alpha\beta} + j\,\delta A\, V_{\alpha\beta} \qquad \to \qquad E^j_\alpha,\ T^j_{\alpha\beta} \tag{S6}$$

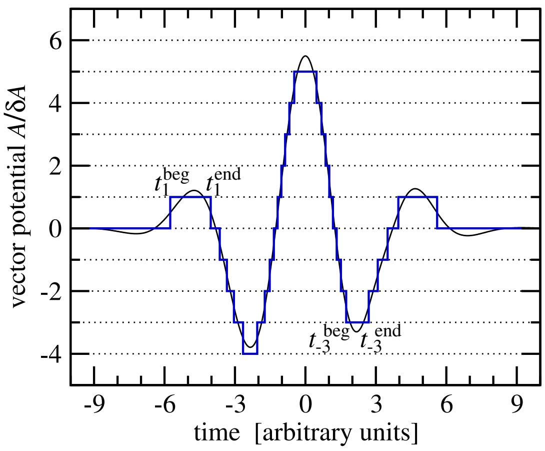


Figure S1: Sketch of the discretization of a time-dependent vector potential $A(t)$ in units of $\delta A$. Two generic time steps $t_j^{\text{beg}} \ldots t_j^{\text{end}}$ are indexed. Note that the step height $\delta A$ here is rather large for visualization purposes.

and calculate by means of the eigenvalues $E_\alpha^j$ and eigenvectors $T_{\alpha\beta}^j$ the corresponding matrices for the time evolution operator

$$U_{\alpha\beta}^j = \sum_\gamma T_{\gamma\alpha}^j e^{-\mathrm{i}E_\gamma^j[t_j^{\mathrm{end}}-t_j^{\mathrm{beg}}]} T_{\gamma\beta}^j \tag{S7}$$

for all $j$. Additionally and similarly important in view of efficiency, the pre-calculated $E_\alpha^j$ and $T_{\alpha\beta}^j$ can be used for all pulses (the fluctuating ones as well as the reference one) for a specific system. Only by this method we were able to calculate millions of spectra, necessary for training the network.

**Physical systems for applications**

On one hand, the number of TDSEs to be solved in the 3D case are considerably lower. On the other hand, a single calculation is more expensive.

**He** In order to calculate the field-free eigenstates we use an effective potential [4]. For angular momenta $\ell = 0 \ldots 4$ we calculated the lowest 2250 states in a box of size $r = 0 \ldots 3\times10^3 \mathrm{a}_0$ with a Numerov step size of $\delta r = 0.01\,\mathrm{a}_0$.

**$H_2^+$** Field-free states and their couplings are calculated in terms of prolate-spheroidal coordinates $\{\xi, \eta\}$, in which the problem separates [5]. The angular domain $-1 \le \xi \le +1$ is described in terms of Legendre polynomials, the radial domain $1\,\mathrm{a}_0 \le \eta \le 2000\,\mathrm{a}_0$ in terms of B-splines. For the coupling we assume that the molecule is aligned with the laser polarization, the orientation with the large dipole matrix elements. The internuclear distance is taken as $R = 2\,\mathrm{a}_0$.

The propagation in time is achieved by direct computation

$$\psi_\alpha(t+\delta t) = \sum_{k=0}^{k_{\max}} \frac{[-\mathrm{i}\,\delta t]^k}{k!} \sum_{\beta_1\ldots\beta_k} H_{\alpha\beta_k}(t+\delta t/2, t)\ldots H_{\beta_2\beta_1}(t+\delta t/2, t)\psi_{\beta_1}(t), \tag{S8}$$

with $k_{\max}$ defined by a sufficiently small contribution, i. e. $\left|\sum_{\beta_1\ldots\beta_k}\ldots\right|^2 < 10^{-30}$. Hereby, $k_{\max}$ may change from step to step.

## 4 Photo-electron spectra

From the solution of the time-dependent Schrödinger equation, i. e. by means of the field-free-state expansion amplitudes $a_\alpha(t)$ for $t \to \infty$, we get the corresponding photo-electron spectrum as

$$P(E) = \sum_\alpha \left|a_\alpha(+\infty)\right|^2 K(E - E_\alpha), \tag{S9}$$

with the kernel function $K(E) = \exp(-E^2/\Delta E^2)/\sqrt{\pi}\Delta E$. We have chosen $\Delta E = 0.2\,\mathrm{eV}$, which is slightly smaller than the typical spacing between the field-free states.

Those spectra are fitted by the $k$ first harmonic oscillator eigenfunctions $\chi_i(E)$ according to

$$P(E) = \left|\sum_{i=0}^{k-1} C_i \chi_i(E)\right|^2. \tag{S10}$$

Those eigenfunctions (normalized by the pre-factor $N_i$) are given by

$$\chi_i(E) = N_i\, \mathrm{e}^{-\Omega_*[E-E_*]^2/2} H_i\left(\sqrt{\Omega_*}[E-E_*]\right), \tag{S11a}$$

$$\text{with } \Omega_* = T_0^2/4\ln 2 \text{ and } E_* = E_0 + 2\omega_*, \tag{S11b}$$

where $H_i$ stands for the $i$th Hermite polynomial. Hereby, the frequency $\Omega_*$ matches the bandwidth of the pulse and the displacement $E_*$ corresponds to the energy reached by a two-photon transition from the ground state. Thus, a weak Gaussian pulse (in perturbation regime) with a duration $T_0$ and a carrier frequency $\omega_*$ would give a photo-electron spectrum that is very similar to $\chi_0(E)$ as defined in Eq. (S11).

## 5 Artificial neural network

We use a fully connected feed-forward artificial neural network to establish a mapping from noisy $\overline{\mathbf{C}}_{kj}$ to noise-free spectra $\mathbf{C}_k^{\text{ref}}$, cf. Fig. 2 in the main text. In our network $\overline{\mathbf{C}}_{kj}$ and $\mathbf{C}_{kj}$ are connected through 7 hidden layers which contain 40 nodes each. They are linked with weights $\mathbf{W}$ and have biases $\mathbf{B}$ and activation functions $\mathbf{f}$. This simple network can be described mathematically as

$$\mathbf{C} = \mathbf{W}_7\mathbf{Y}_7 + \mathbf{B}_7, \quad \mathbf{Y}_{7-k} = \mathbf{f}_{7-k}\big(\mathbf{W}_{6-k}\mathbf{Y}_{6-k} + \mathbf{B}_{6-k}\big) \text{ with } k=0\ldots6, \quad \mathbf{Y}_0 = \overline{\mathbf{C}}. \tag{S12}$$

In the above equations $\mathbf{W}_k$ represents weights connecting $k$th layer neurons with $(k+1)$th layer neurons and $\mathbf{B}_k$ stands for biases linked to $(k+1)$th layer neurons. The dimensions of $\mathbf{Y}_k$, $\mathbf{W}_k$ and $\mathbf{B}_k$ are $n_k$, $n_{k+1}\times n_k$ and $n_{k+1}$, respectively, where $n_k$ is the number of $k$th layer neurons. (The activation functions $\mathbf{f}_{k+1}$ are to be understood as $n_k$-dimensional functions.) Note that input and output layer dimensions are $n_{\text{bas}} = 60$ and $n_{\text{bas}} = 40$ respectively, the number of basis functions to represent the photoelectron spectra. The total number of trainable parameters in the network (S12) is 13,920. We use *ReLU* [6], i. e. $f(x) = \max(0, x)$, as activation function to introduce the non-linearity in the connection for all hidden layers. Note that this functional value does not saturate for very large value of $x$.

For the initial choice of random weights and biases, we use the so-called XAVIER initialization [7], where random weights are considered from a normal distribution with zero mean and a variance of $2/[n_k+n_{k+1}]$, where $n_k$ is the number of neurons at $k$th layer. Such an initialization reduces the possibility to drive the network into saturated states and accelerates convergence. All biases $\mathbf{B}$ are set to 1 initially. The weights and biases of the network (S12) are obtained using the ADAM optimization algorithm [8], which is very efficient for stochastic optimization that is based on an adaptive-learning method by which it computes individual learning rates for each weight and the biases in the network. We use the same values for the parameters $\beta_1$, $\beta_2$, $\alpha$, and $\varepsilon$ as the ones given in "Algorithm 1" in the original paper on the ADAM method [8].

In order to reduce the computational cost, we applied mini-batch optimization [9] with the batch size being 500 and introduced early stopping with a patience of 35 (the number of epochs with an increasing cost function on the validation data). Typically we had to run about 100 epochs in order to train the network. On a single batch, a forward pass and a backward pass is a single iteration. Each epoch covers all training samples once. For a total sample size of $1.6\times10^5$ and a batch size of 500 we need 320 iterations to complete a single epoch. To reduce the complexity of the network during the training we drop some neurons with a dropping rate 0.1 [10].

### Training-data size

The value of the cost function [Eq. (4) in the main text] as well as the average difference [Eq. (5) Ibid.] decrease logarithmically with the training-data size as shown for validation data set in Fig. S2. The figure shows also that along with the mean, obtained from several optimization runs for the network, the standard deviation among those runs decreases.

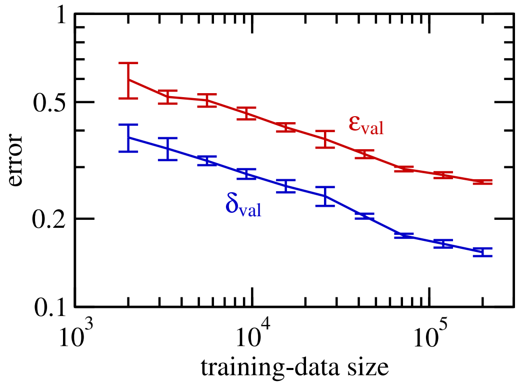


Figure S2: Predicted performance by the validation data measured with the cost function $\delta_{\text{val}}$ [Eq. (4)] and the absolute error $\varepsilon_{\text{val}}$ [Eq. (5)] as a function of the size $n$ of pairs of spectra contained in the complete SHM data set.

## References


[1] T. Pfeifer, Y. Jiang, S. Düsterer, R. Moshammer, and J. Ullrich, *Partial-coherence method to model experimental free-electron laser pulse statistics*. Opt. Lett. **35**, 3441 (2010).

[2] G. Geloni, E. Saldin, L. Samoylova, E. Schneidmiller, H. Sinn, Th Tschentscher, and M. Yurkov, *Coherence properties of the European XFEL*. New J. Phys. **12**, 035021 (2010).

[3] G. M. Nikolopoulos and P. Lambropoulos, *Effects of free-electron-laser field fluctuations on the frequency response of driven atomic resonances*. Phys. Rev. A **86**, 033420 (2012).

[4] X. M. Tong and C. D. Lin, *Empirical formula for static field ionization rates of atoms and molecules by lasers in the barrier-suppression regime*. J. Phys. B **38**, 2593 (2005).

[5] L. D. Landau and E. M. Lifschitz, *Quantum mechanics*. Pergamon Press, Oxford 1989.

[6] X. Glorot, A. Bordes, and Y. Bengio, *Deep sparse rectifier neural networks*. PMLR **15**, 315 (2011).

[7] X. Glorot and Y. Bengio, *Understanding the difficulty of training deep feedforward neural networks*. PMLR **9**, 249 (2010).

[8] D. P. Kingma and J. L. Ba, *ADAM: A method for stochastic optimization*. arXiv:1412.6980 [cs] (2017).

[9] M. Li, T. Zhang, Y. Chen, and A. J. Smola, *Efficient mini-batch training for stochastic optimization* in *Proceedings of the 20th ACM SIGKDD Conference*, 661 (2014).

[10] N. Srivastava, G. Hinton, A. Krizhevsky , I. Sutskever, and R. Salakhutdinov, *Dropout: A simple way to prevent neural networks from overfitting*. JMLR **15**, 1929 (2014).
